# Supplementary material for: Unifying Homophily and Heterophily Network Transformation via Motifs
Source: arXiv:2012.11400 source file (2020-12-27)
Supplement: Supplementary file 1 [file Appendix.tex]

\newpage
\section{Appendix}
We first introduce planted partition model as follows:
\begin{Definition}
(Planted Partition Model) Let $G \sim G(nk, k, p, q)$ be a graph sampled from the planted partition model on $nk$
vertices, with $k$ clusters $C = 
\{C_1, \cdots, C_i, \cdots, C_k\}$ each with exactly $n$
vertices. The edge set is then sampled at random as follows:
two vertices $\{v_i,v_j\}\in C_i$ are connected with probability $p$ otherwise with
probability $q<p$.
\end{Definition}

The below lemma show a relation between homophily and proximity.
\begin{lemma}\label{lemma:relation}
Let $G \sim G(nk, k, p, q)$ be an unweitghted graph  with $k$ clusters
$C = \{C_1, \cdots, C_i, \cdots, C_k\}$, nodes \{$v_i,v_j\}\in C_s$ and 
$v_k \in C_t$, the expectation value of $l$-order proximity between $v_i$ and $v_j$  is $\mathbb{E}[a_{ij}^{(l)}]$, 
Then,
\begin{eqnarray}
\mathbb{E}[a_{ik}^{(l)}] < \mathbb{E}[a_{ij}^{(l)}] \label{equ:ADJ}
\end{eqnarray}
\begin{eqnarray}
\mathbb{E}[p_{ik}^{(l)}] < \mathbb{E}[p_{ij}^{(l)}]\label{equ:RW}
\end{eqnarray}
\end{lemma}

\begin{proof}
\begin{equation*}
\mathbb{E}[a_{ij}^{(l)}] = \sum_{z=1}^{kn}\mathbb{E}[a_{iz}^{(l-1)}] \cdot \mathbb{E}[a_{zj}]
\end{equation*}
\begin{equation*}
\mathbb{E}[p_{ik}^{(l)}] = \sum_{z=1}^{kn}\mathbb{E}[p_{iz}^{(l-1)}] \cdot \mathbb{E}[p_{zk}]
\end{equation*}
The above equation interpret the proximity that it is
going from node $v_i$ to node $v_j$ in $l$ steps 
is obtained by summing the proximity of the mutually events of going from node $i$ to
some node $v_k$ in the first $n-1$ walk steps and then going from node $k$ to node $j$ 
in the $l$th walk step. 
For notation brevity, let $\mathbb{E}[\cdot] =\cdot$, so
% $\forall \{v_r, v_s\} \in V, 1\le h\le l$
\begin{eqnarray*}
a_{ij}^{(l)}- a_{ik}^{(l)} =  \sum_{z=1}^{kn}a_{iz}^{(l-1)} \cdot (a_{iz}-a_{zk}) \\
= \sum_{z \in C_s} a_{iz}^{(l-1)} \cdot (a_{iz}-a_{zk}) + \sum_{z \in C_t} a_{iz}^{(l-1)} \cdot (a_{iz}-a_{zk}) \\+ \sum_{ z \in\{ C_h| 1\leq h\leq k, h \notin \{s,t\}\}} a_{iz}^{(l-1)} \cdot (a_{iz}-a_{zk})\\
= \sum_{z \in C_s} a_{iz}^{(l-1)} \cdot (p-q) - \sum_{z \in C_t} a_{iz}^{(l-1)} \cdot (p-q)
\end{eqnarray*}
Then, according to Lemma \ref{lemma:ntimes1} and Lemma \ref{lemma:ntimes2},
\begin{equation*}
    \sum_{z \in C_t} a_{iz}^{(l-1)} = na_{ij}^{(l-1)},
\end{equation*}
\begin{equation*}
\sum_{z \in C_s} a_{iz}^{(l-1)} = na_{ik}^{(l-1)},
\end{equation*}
so,
\begin{eqnarray*}
a_{ij}^{(l)}- a_{ik}^{(l)} = (p-q)(na_{ij}^{(l-1)}-na_{ik}^{(l-1)})
\\=n^{l-1}(p-q)^{l-1}(a_{ij}-a_{ik})=n^{l-1}(p-q)^l>0.
\end{eqnarray*}

\end{proof}

\begin{lemma} \label{lemma:ntimes1}
Let $G \sim G(nk, k, p, q), \{v_i, v_r, v_s\} \in C_s$, then we have $\mathbb{E}[a_{id}^{(h)}] = \mathbb{E}[a_{ie}^{(h)}]$. 
\end{lemma}
\begin{proof}
For notation brevity, let $\mathbb{E}[\cdot] =\cdot$, so
\begin{eqnarray*}
a_{id}^{(h)}-a_{ie}^{(h)} = \sum_{z=1}^{kn} a_{iz}^{(h-1)}\cdot a_{zd} 
- \sum_{z=1}^{kn} a_{iz}^{(h-1)}\cdot a_{ze}\\
= \sum_{z=1}^{kn} a_{iz}^{(h-1)} \cdot (a_{zj}-a_{ze}) 
= \sum_{z \in C_s} a_{iz}^{(h-1)} \cdot (a_{zj}-a_{ze})\\ + \sum_{z \in\{ C_h| 1\leq h\leq k, h \neq s\}}a_{iz}^{(h-1)} \cdot (a_{zj}-a_{ze}) = 0
\end{eqnarray*}
\end{proof}

\begin{lemma}\label{lemma:ntimes2}
Let $G \sim G(nk, k, p, q), v_i \in C_s, \{v_r, v_s\} \in C_t$, we have $\mathbb{E}[a_{ir}^{(h)}] = \mathbb{E}[a_{is}^{(h)}]$. 
\end{lemma}
\begin{proof}
For notation brevity, let $\mathbb{E}[\cdot] =\cdot$, so
\begin{eqnarray*}
a_{ir}^{(h)}-a_{is}^{(h)} = \sum_{z=1}^{kn} a_{iz}^{(h-1)}\cdot a_{zr} 
- \sum_{z=1}^{kn} a_{iz}^{(h-1)}\cdot a_{zs}\\
= \sum_{z=1}^{kn} a_{iz}^{(h-1)} \cdot (a_{zr}-a_{zs}) 
= \sum_{z \in C_t} a_{iz}^{(h-1)} \cdot (a_{zr}-a_{zs})\\ + \sum_{z \in\{ C_h| 1\leq h\leq k, h \neq t\}} a_{iz}^{(h-1)} \cdot (a_{zr}-a_{zs}) = 0
\end{eqnarray*}
\end{proof}

\subsection{Relation between Homophily and Motif Representation} 

\begin{lemma} \label{lemma:motif_homo}
Let $G \sim G(nk, k, p, q)$ be a unweitghted graph, $\{v_i,v_j\}\in C_i$ and 
$\{v_k\} \in C_j$, and $\{v_i,v_j\}\in E, \{v_i,v_k\}\in E$. 
we use $\mathbb{E}[w(v_i, v_j)]$ to indicate the expected number of triangle  containing the node pair $\{v_i,v_j\}$, then 
\begin{eqnarray}
\mathbb{E}[w(v_i, v_k)] < \mathbb{E}[w(v_i, v_j)]
\end{eqnarray}
\end{lemma}
\begin{proof}
For the case of the edge $\{v_i,v_j\}$:
\begin{equation}
\mathbb{E}[w(v_i, v_j)]=(n-2) p^{2}+(k-1) n q^{2},
\end{equation}
The first term $(n-2) p^{2}$ corresponds to triangles where the third vertex is in the
same component as $v_i$ or $v_j$, the second term $(k-1) n q^{2}$ to triangle where the
third vertex is in another component.

For the case of edge $\{v_i,v_k\}$:

\begin{equation}
    \mathbb{E}[w(v_i, v_k)]=2(n-1) p q+(k-2) n q^{2}
\end{equation}
The first term $2(n-1) p q$ corresponds to triangles where the third vertex is in the
same component as $v_i$or $v_k$, the second term $(k-2) n q^{2}$ to triangle where the
third vertex is in another component.
For simplicity we avoid lower order terms as asymptotically the difference does not
matter. Thus the difference between $\mathbb{E}[w(v_i, v_j)]$
and $\mathbb{E}[w(v_i, v_k)]$

\begin{eqnarray*}
 \mathbb{E}[w(v_i, v_j)] - \mathbb{E}[w(v_i, v_k)] =\\ n p^{2}+(k-1) n q^{2} - 
 2 n p q-(k-2) n q^{2} = n(p-q)^2>0
\end{eqnarray*}
\end{proof}

% \begin{Definition}(Community-Aware Proximity).
% Let $G \sim G(nk, k, p, q)$ be a unweitghted graph  with $k$ clusters
% $\{C_1, \cdots, C_i, \cdots, C_k\}$, nodes $v_i,v_j\in C_i$ and 
% $v_k \in C_j$, the expectation value of $l$-order proximity $\mathbb{E}[s_{ij}^{(l)}]$ is
% larger than the value of $l$-order proximity $\mathbb{E}[s_{ik}^{(l)}]$. It causes 
% the distance of embedding space of $v_i,v_j$ is closer than that of $v_i,v_k$ 
% (reason is that $\mathbb{E}[s_{ij}^{(l)}]$ is large request embedding of $v_i, v_k$ 
% is similar. $\mathbb{E}[s_{ij}^{(l)}]$ (physical meaning is the 
% project from $v_j$ to $v_i$) is the dot product of $v_i, v_k$, only similar
% vector can produce large value (projection results)). 
% \end{Definition}
